# Supplementary material for: Flavoured jet algorithms: a comparative study
Source: arXiv:2506.13449 source file (2025-09-18)

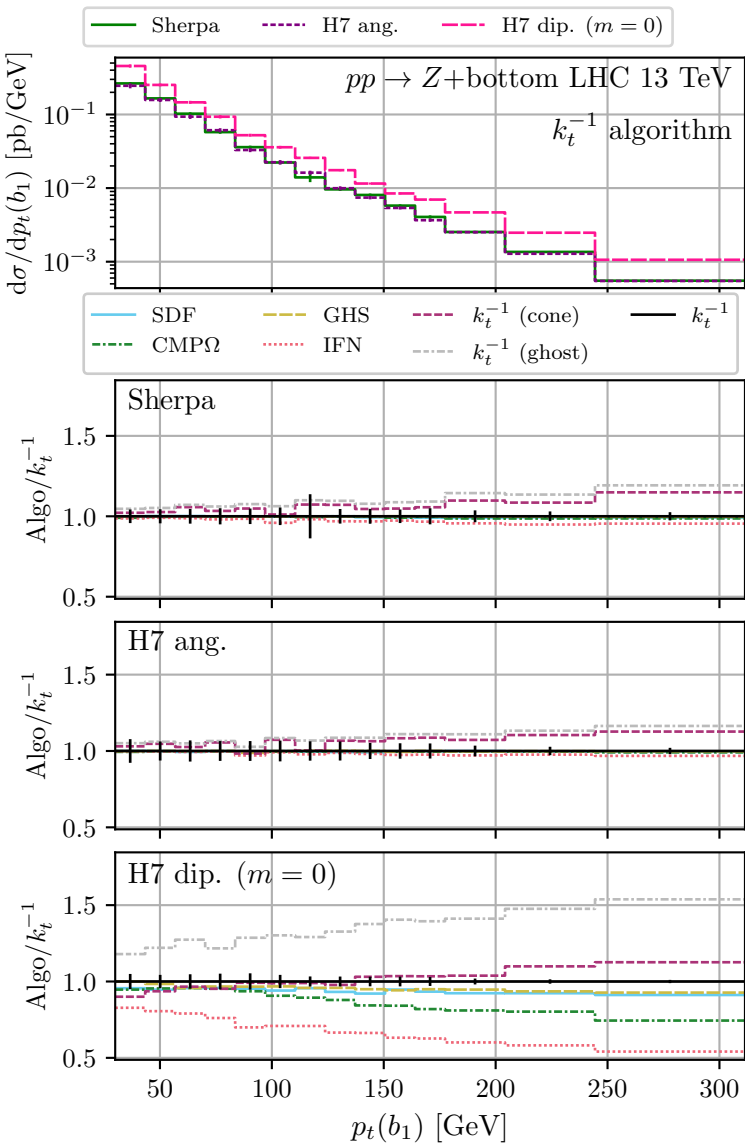

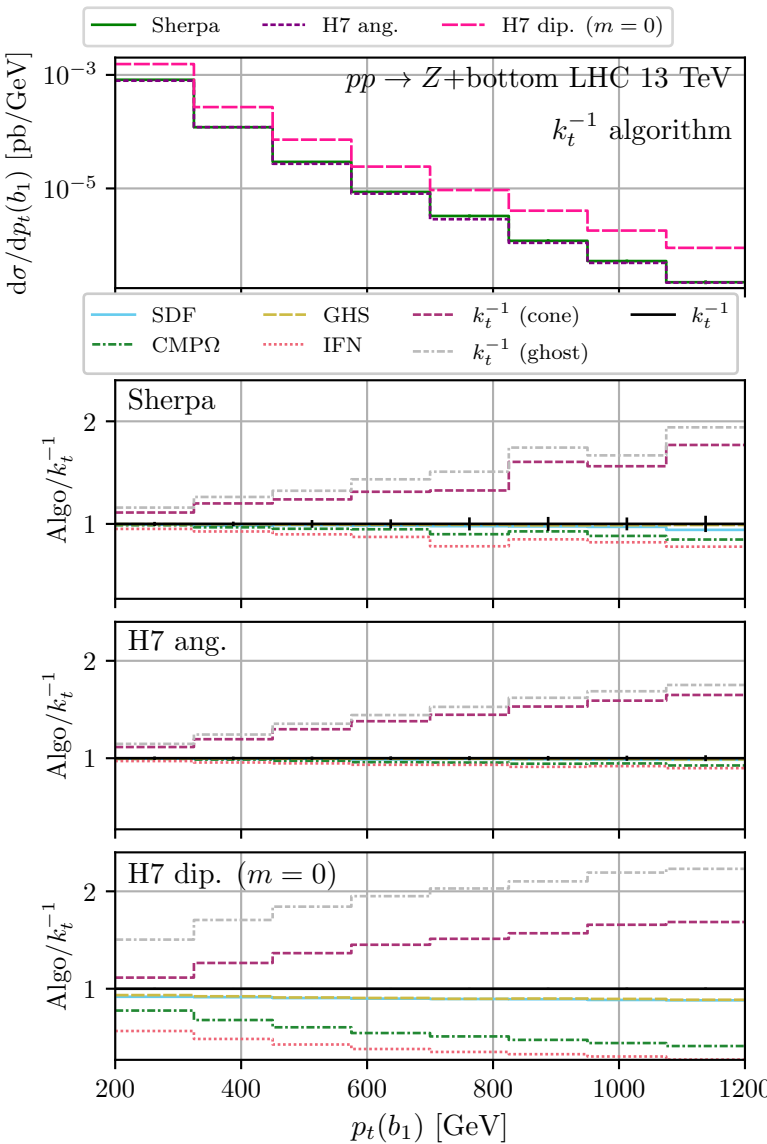

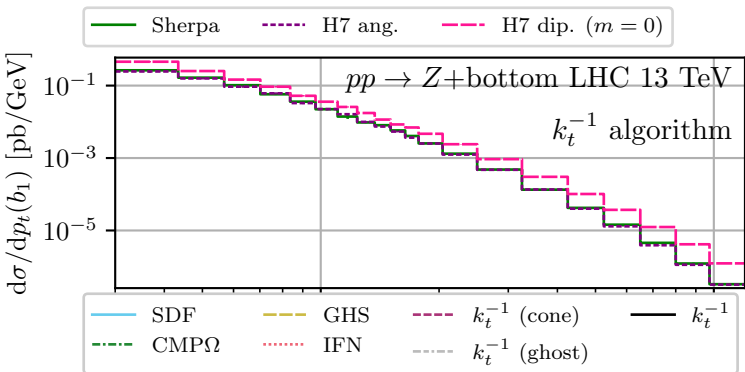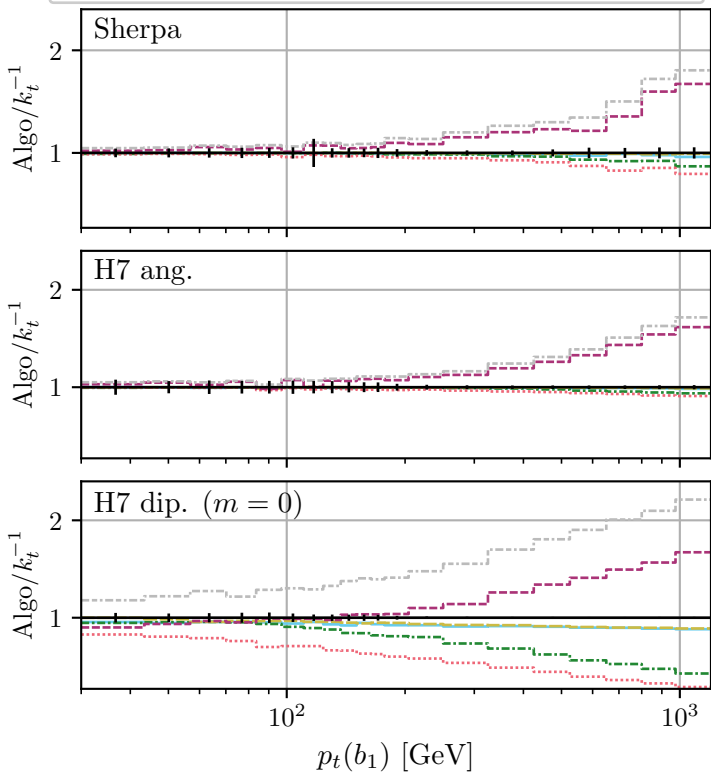

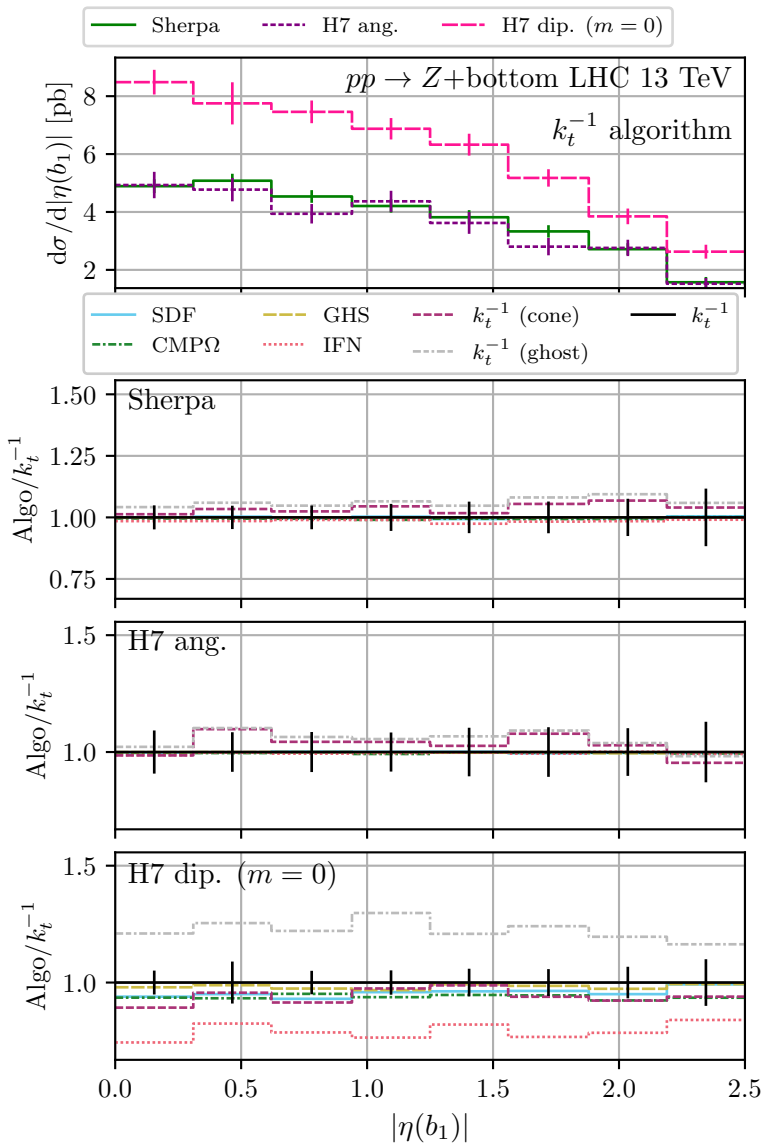

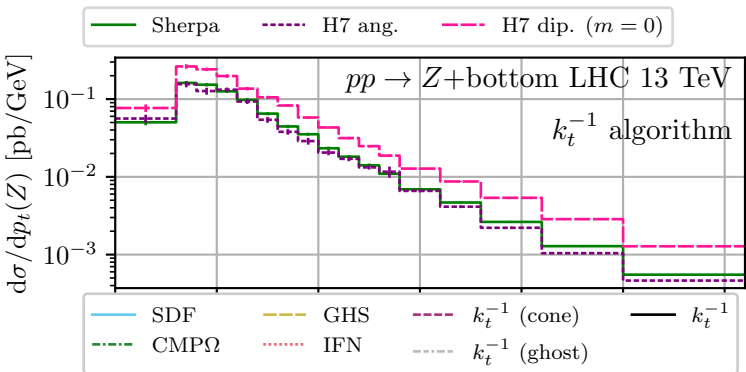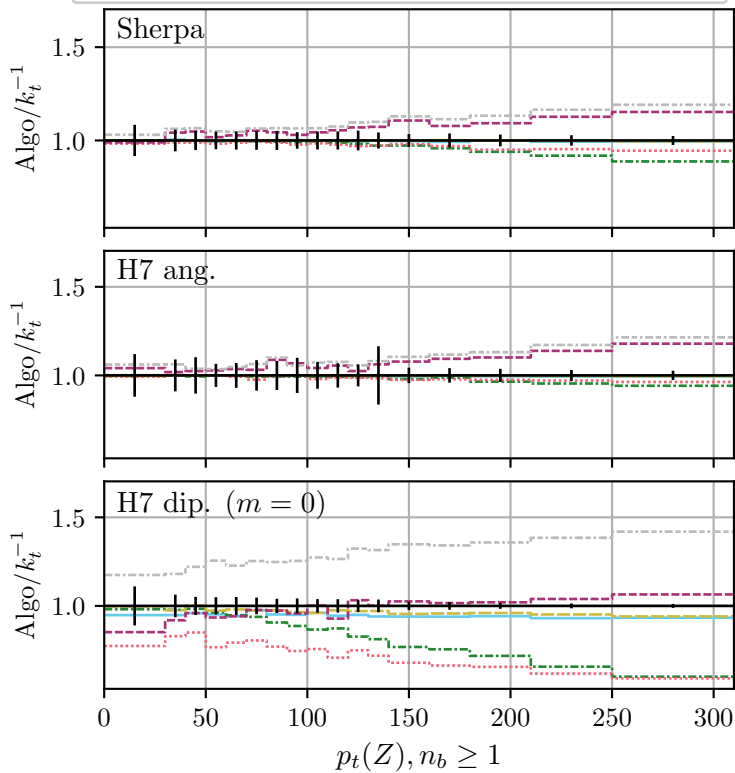

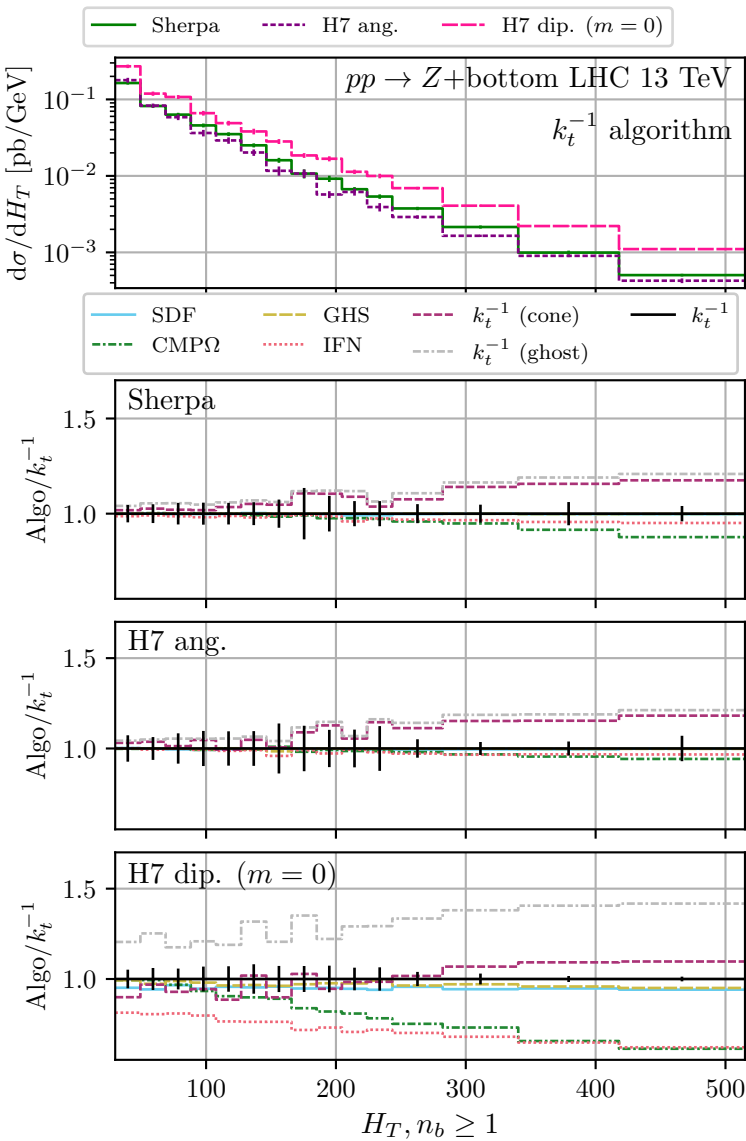

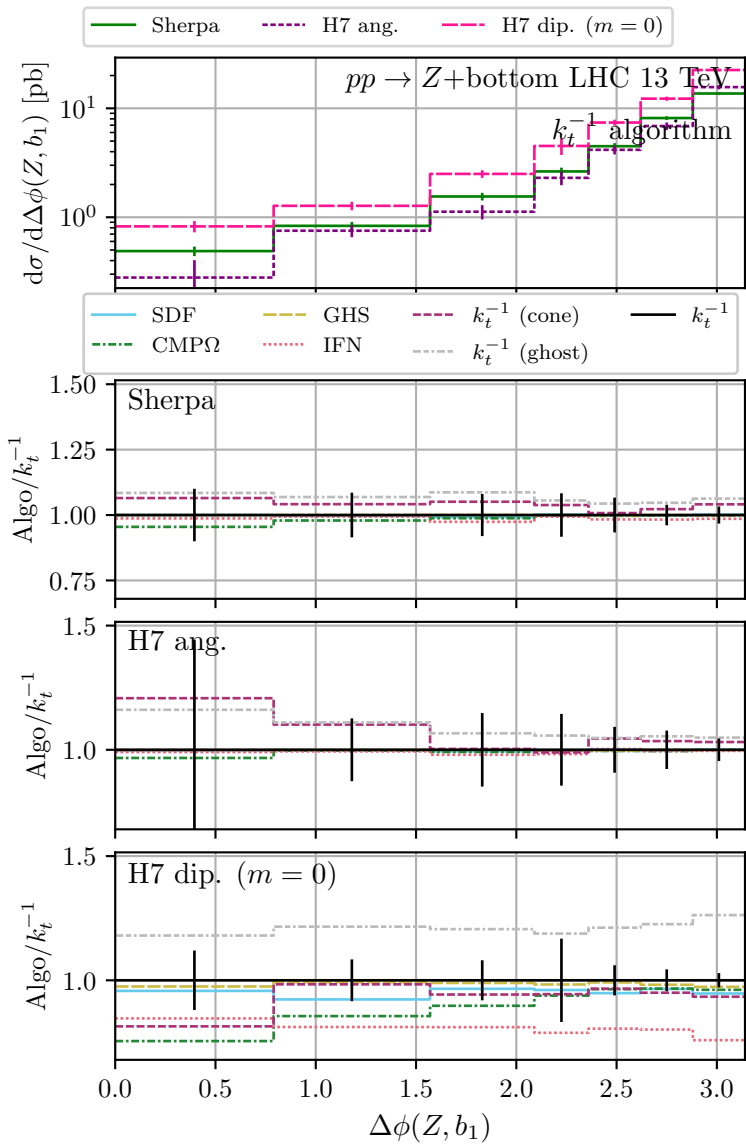

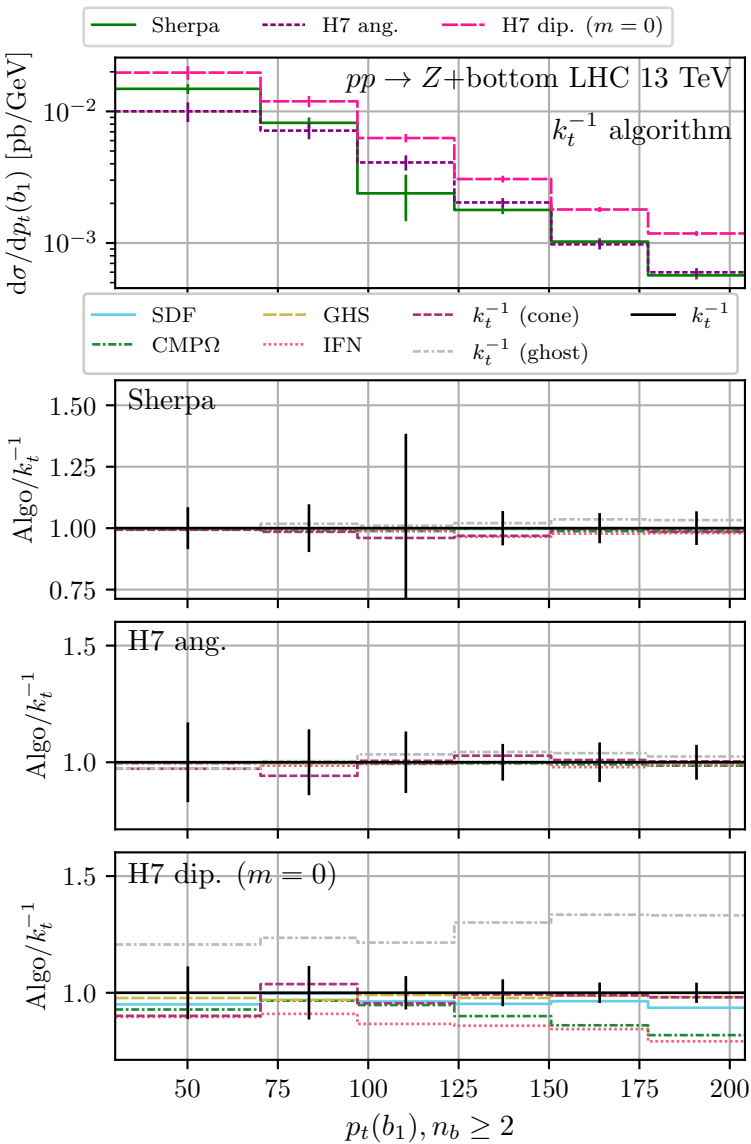



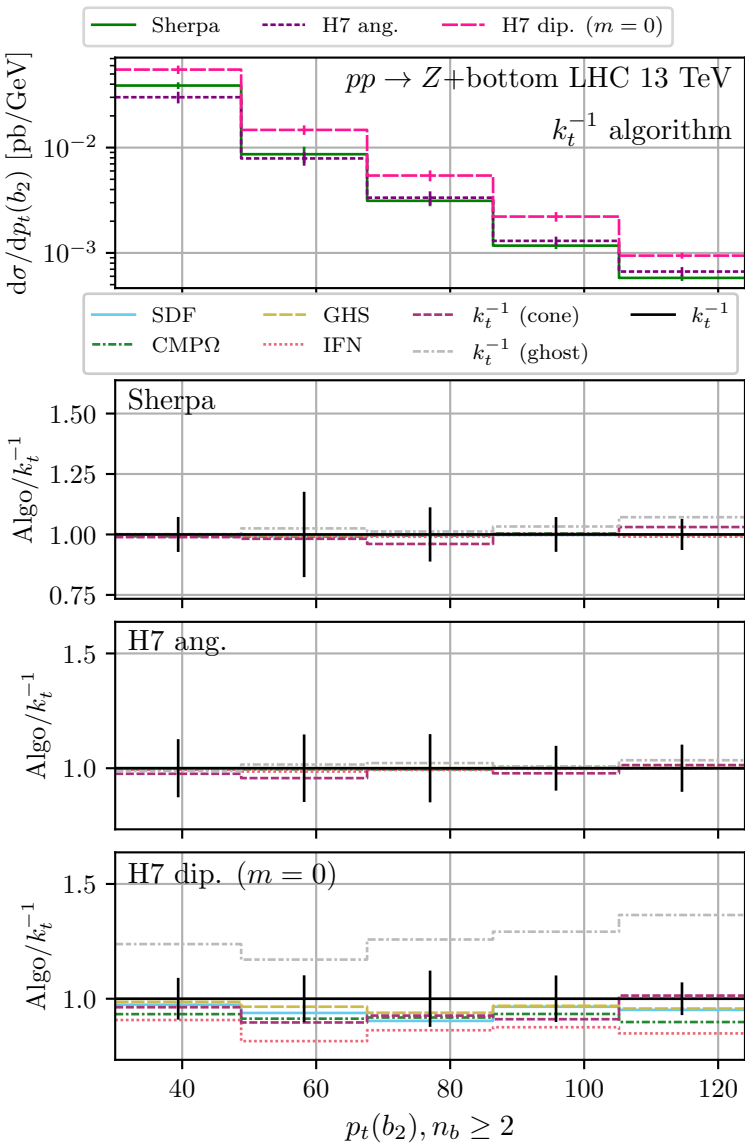

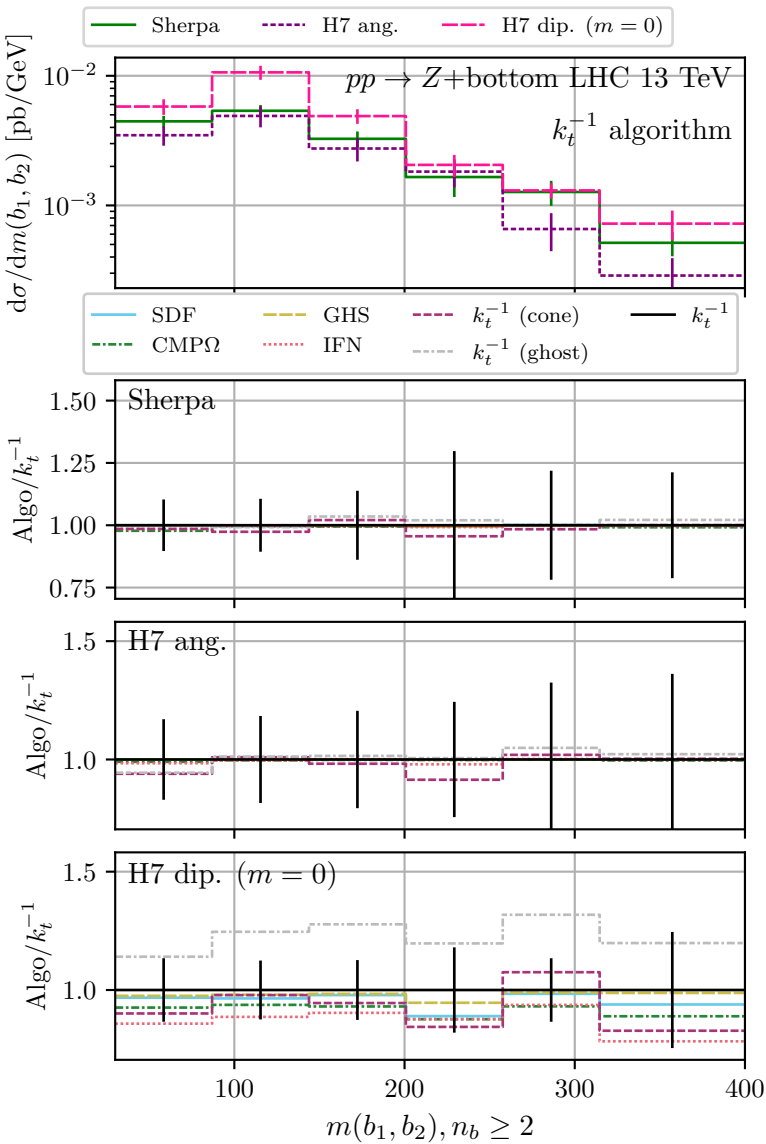

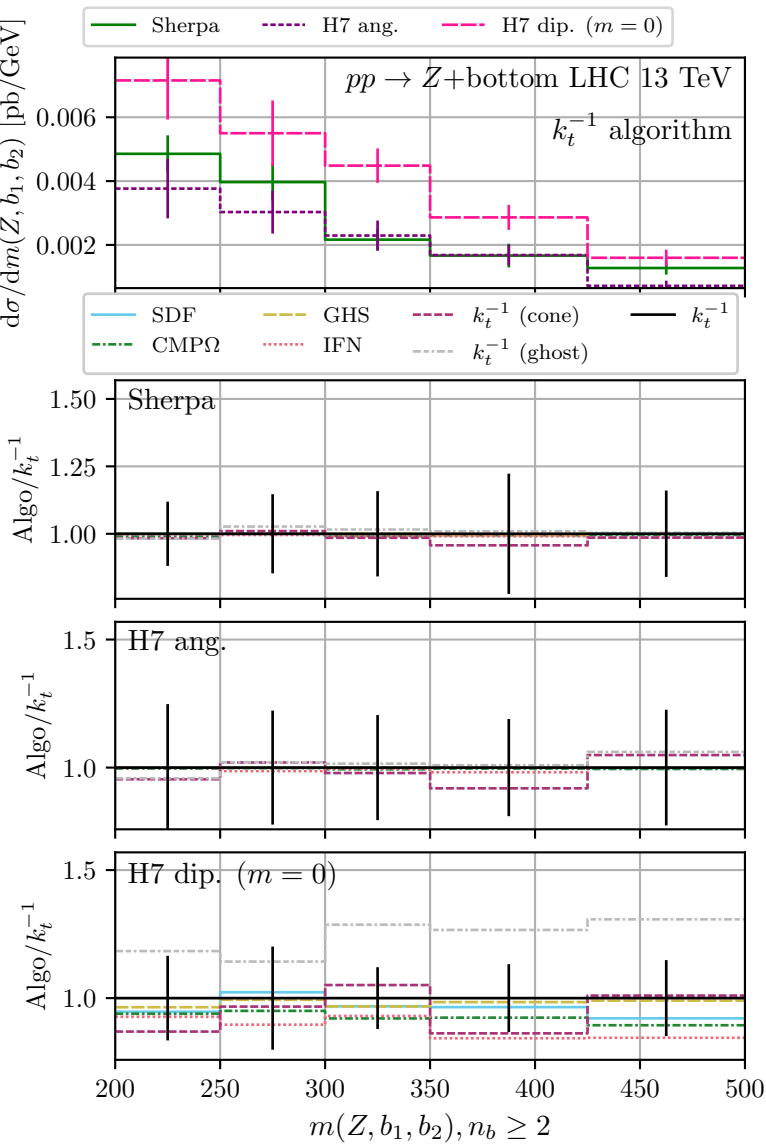

— Sherpa    - - - H7 ang.    - - - H7 dip. ( $m = 0$ )

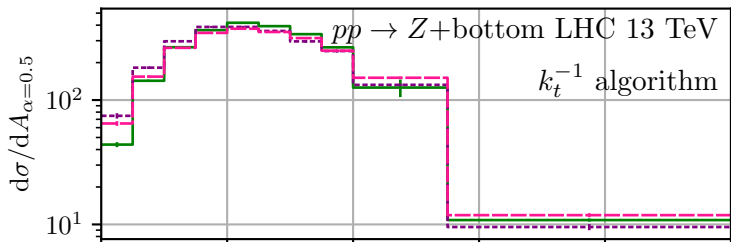

— SDF    - - - GHS    - - -  $k_t^{-1}$  (cone)    —  $k_t^{-1}$   
 - - - CMP $\Omega$     - - - IFN    - - -  $k_t^{-1}$  (ghost)

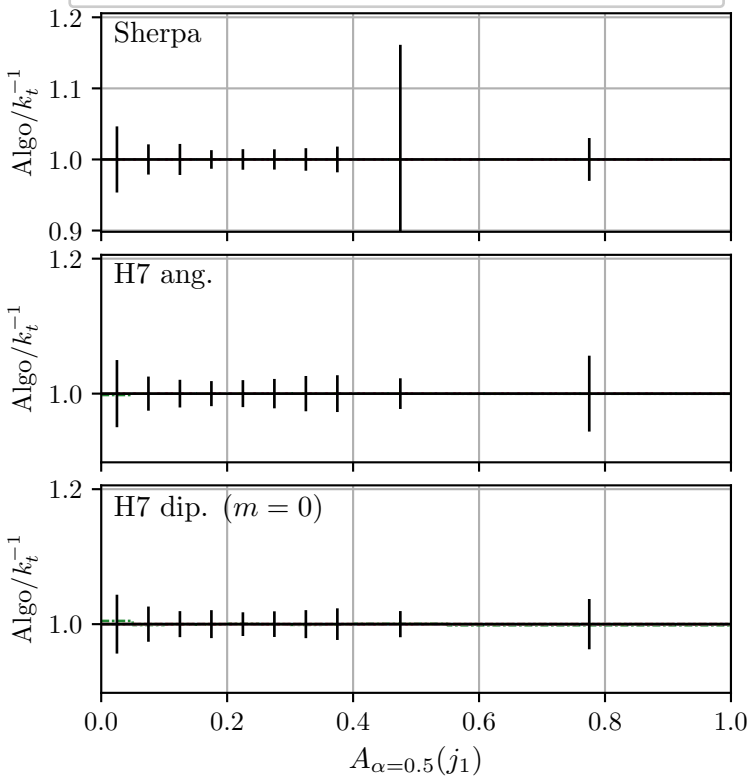

— Sherpa    - - - H7 ang.    - - - H7 dip. ( $m = 0$ )

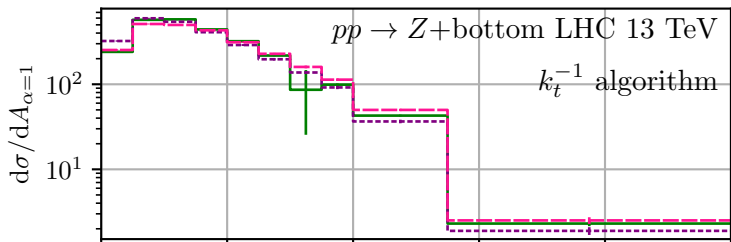

— SDF    - - - GHS    - - -  $k_t^{-1}$  (cone)    —  $k_t^{-1}$   
 - - - CMPΩ    - - - IFN    - - -  $k_t^{-1}$  (ghost)

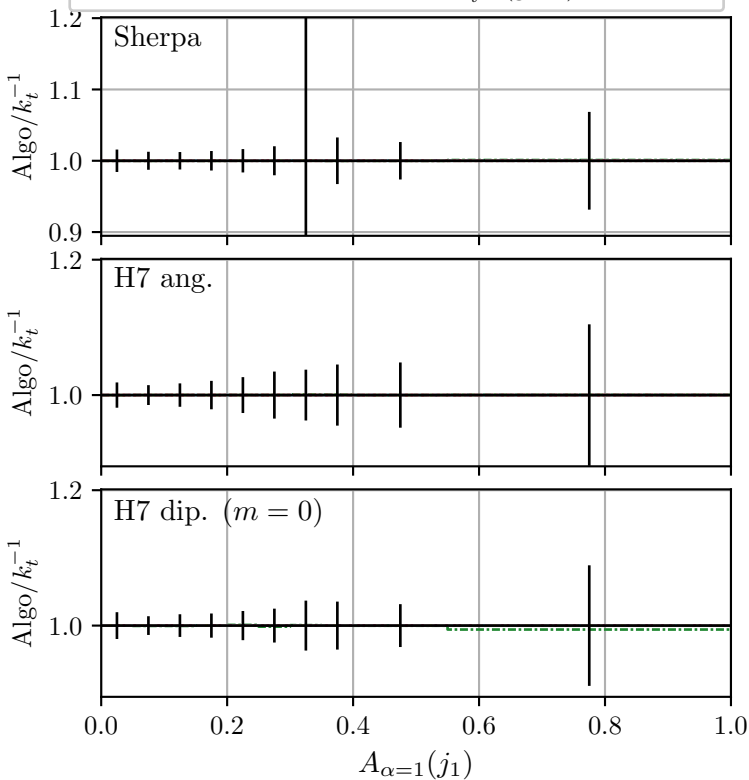

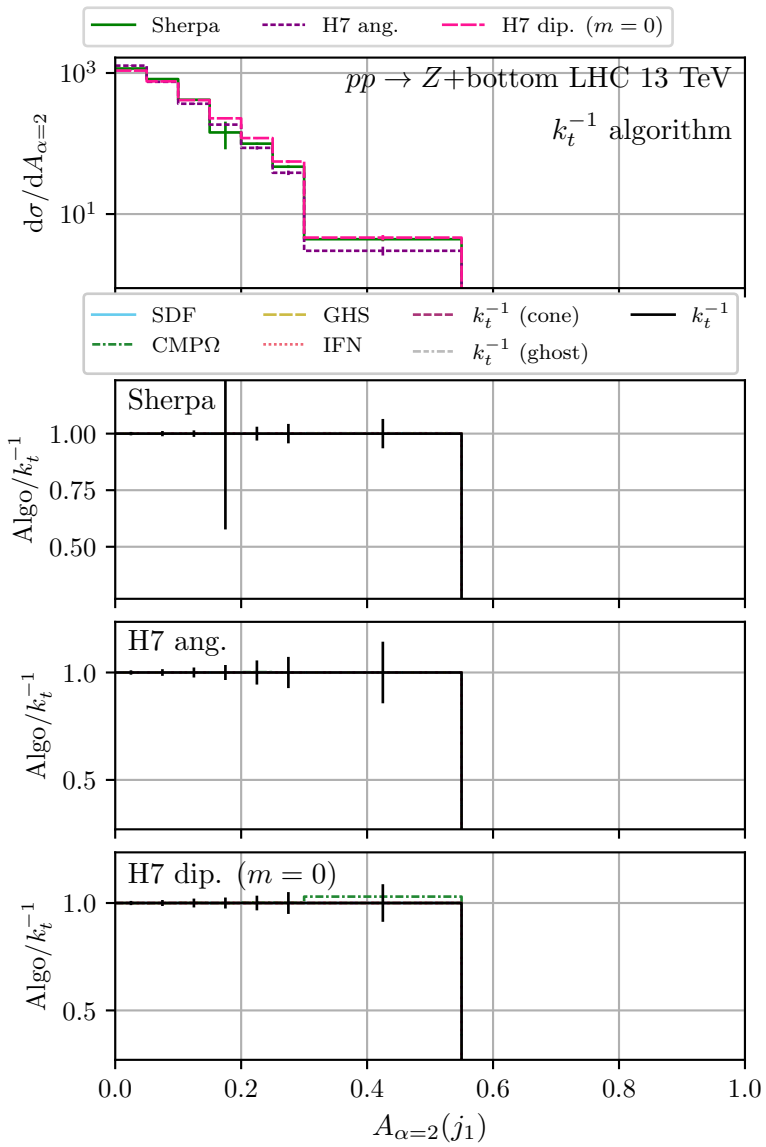

— Sherpa      - - - H7 ang.      - - - H7 dip. ( $m = 0$ )

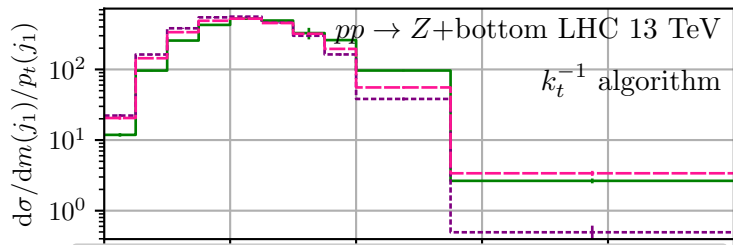

— SDF      - - - GHS      - - -  $k_t^{-1}$  (cone)      —  $k_t^{-1}$

- - - CMP $\Omega$       ····· IFN      - - -  $k_t^{-1}$  (ghost)

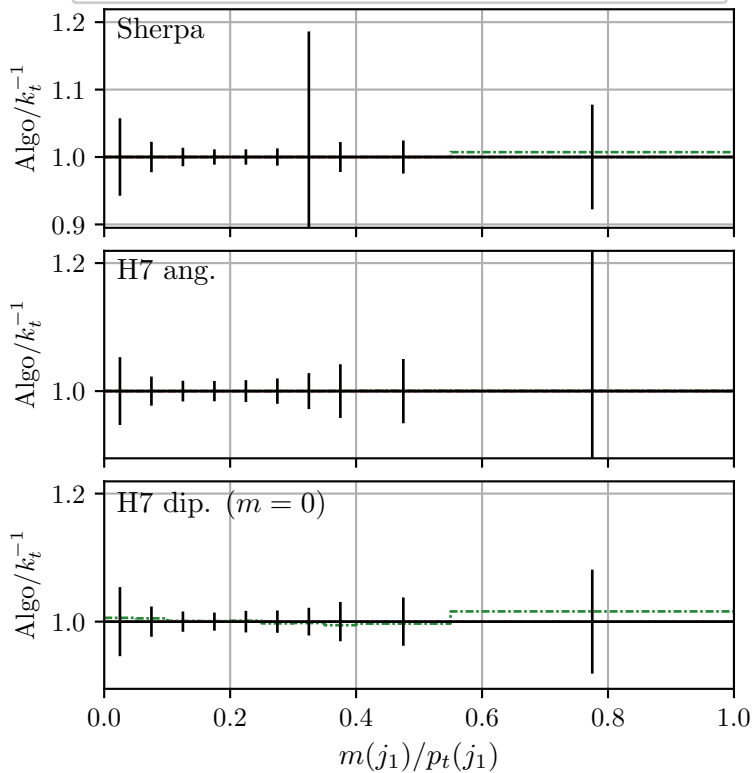

— Sherpa    - - - H7 ang.    - - - H7 dip. ( $m = 0$ )

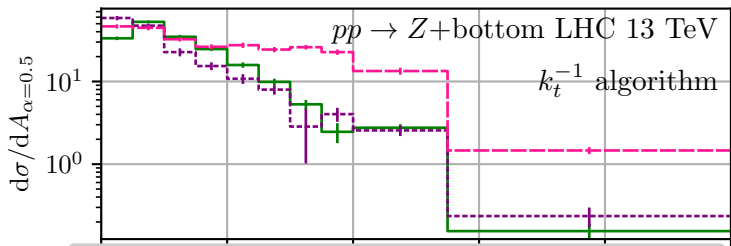

— SDF    - - - GHS    - - -  $k_t^{-1}$  (cone)    —  $k_t^{-1}$   
 - - - CMPΩ    - - - IFN    - - -  $k_t^{-1}$  (ghost)

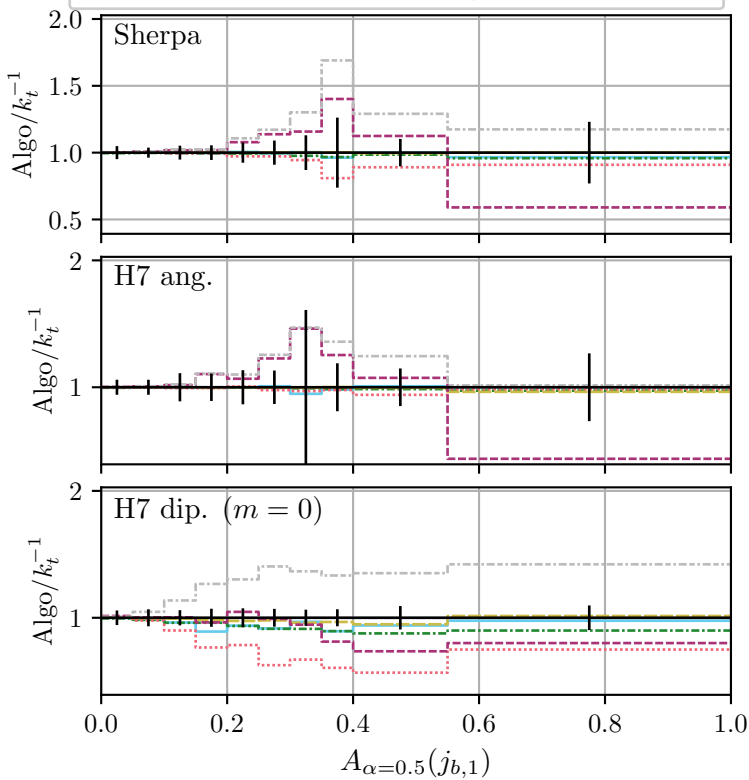



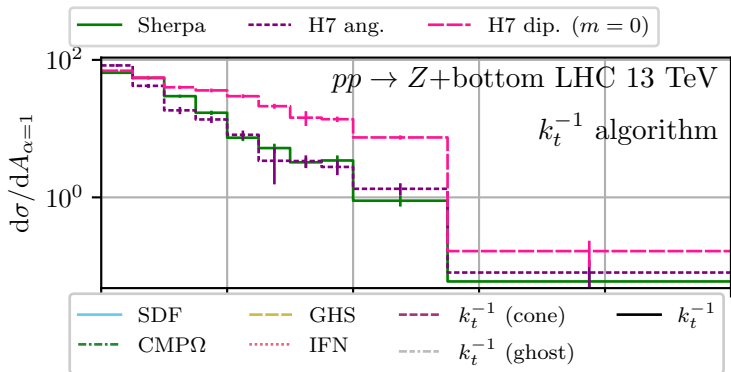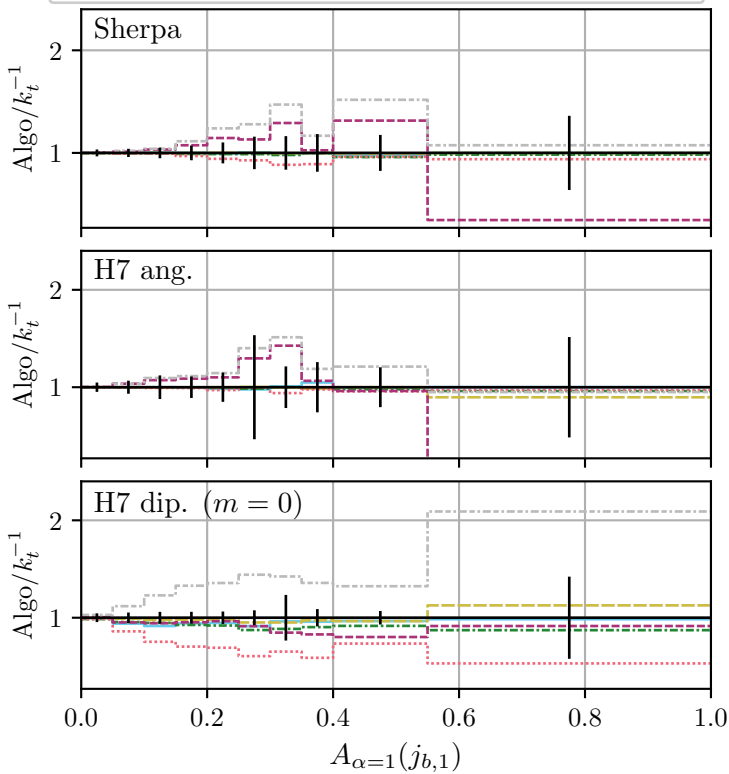

— Sherpa      - - - H7 ang.      - - - H7 dip. ( $m = 0$ )

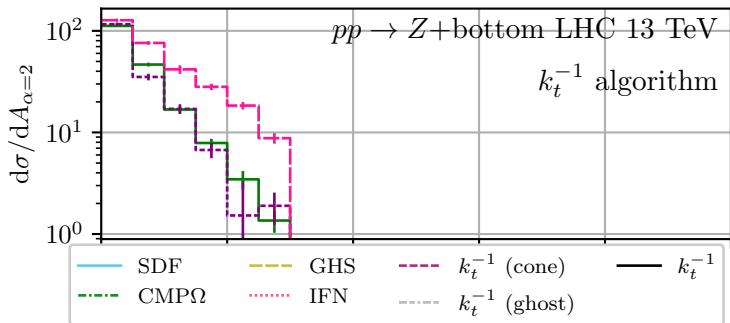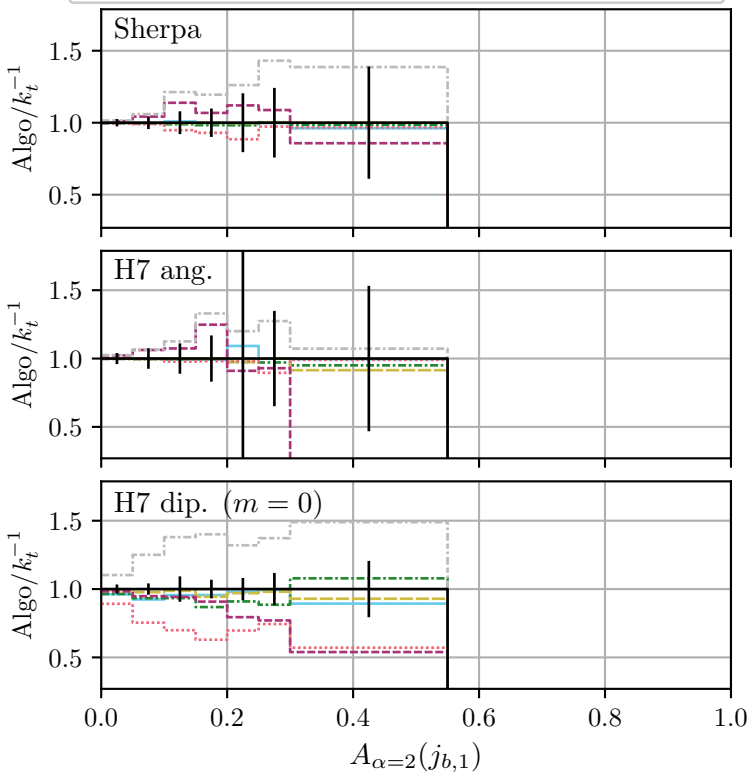

— Sherpa    - - - H7 ang.    - - - H7 dip. ( $m = 0$ )

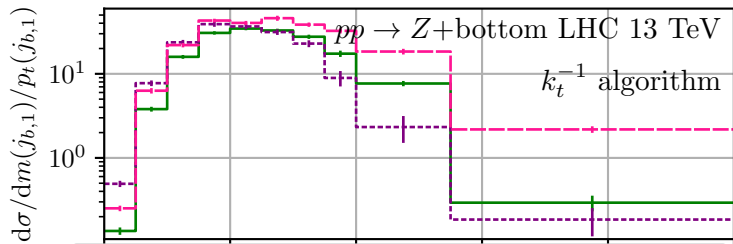

— SDF    - - - GHS    - - -  $k_t^{-1}$  (cone)    —  $k_t^{-1}$   
 - - - CMPΩ    - - - IFN    - - -  $k_t^{-1}$  (ghost)

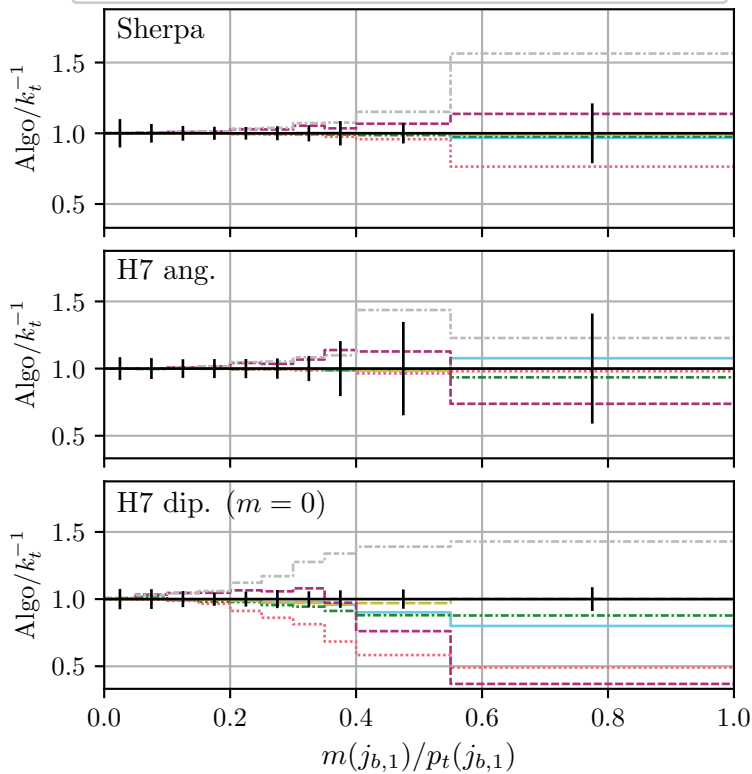

Supplement: Supplementary file 1 [file ppzj_bottom_nlops_comparisons_appendix.pdf]
