# Supplementary material for: Flavoured jet algorithms: a comparative study
Source: arXiv:2506.13449 source file (2025-09-18)

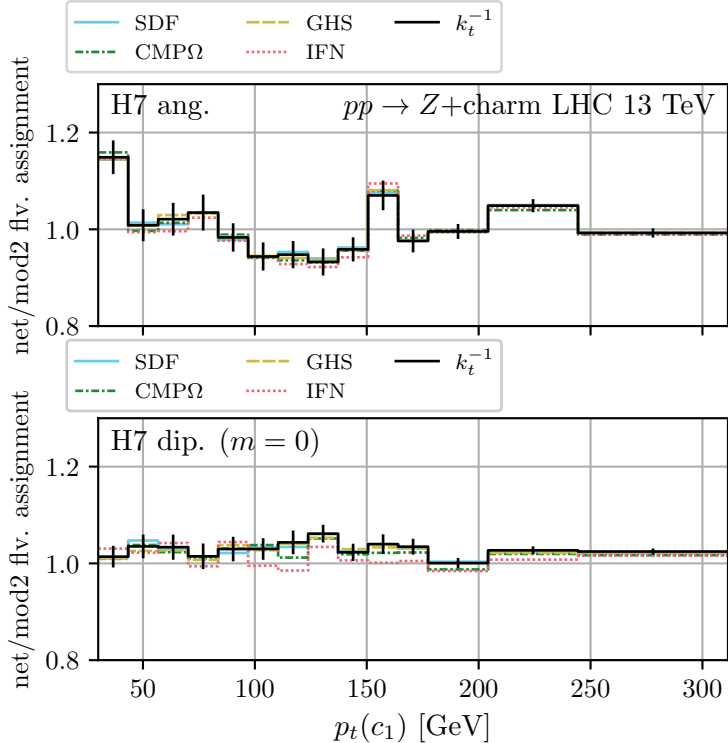

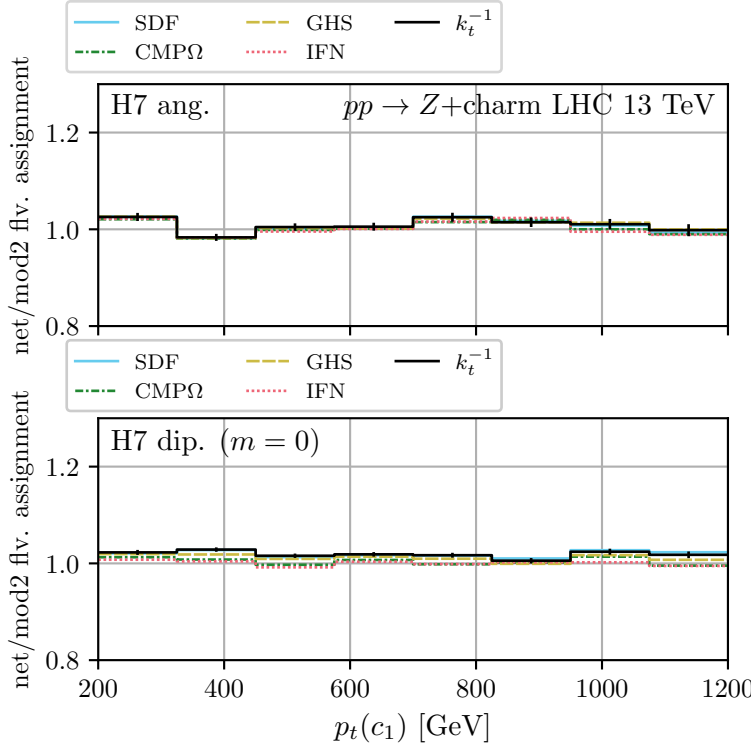

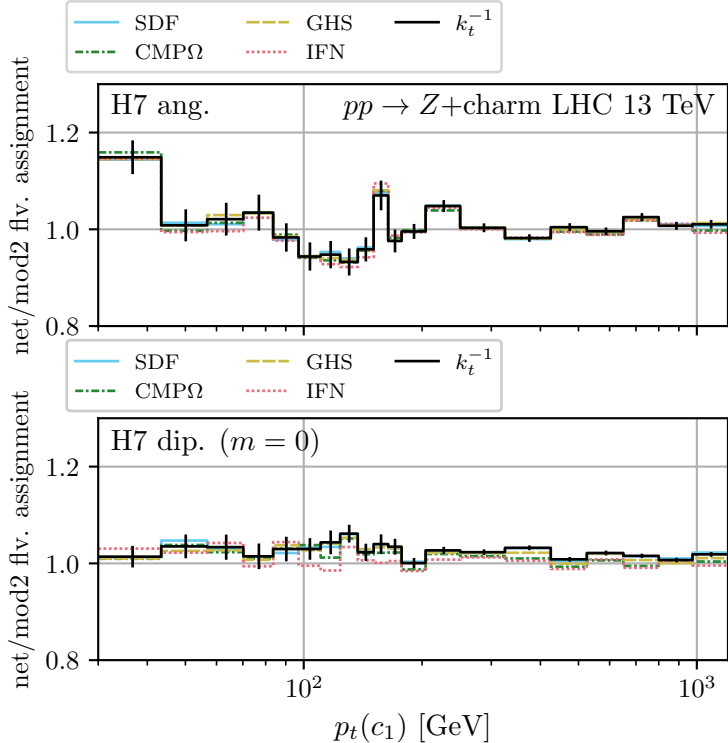

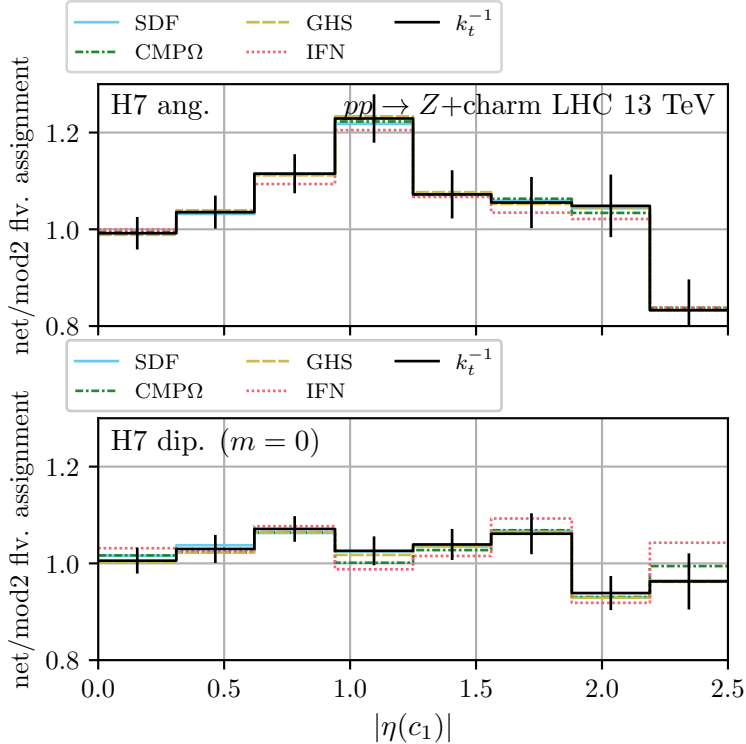

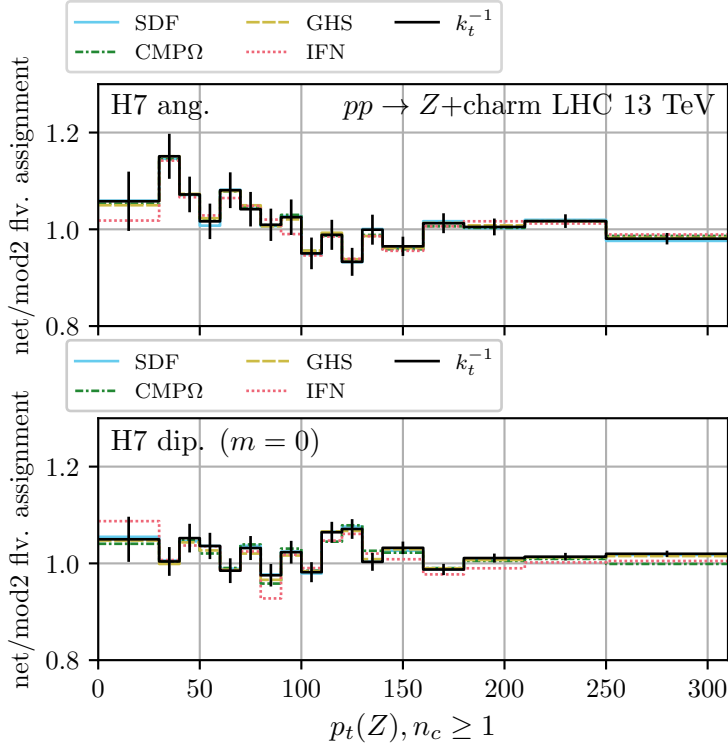

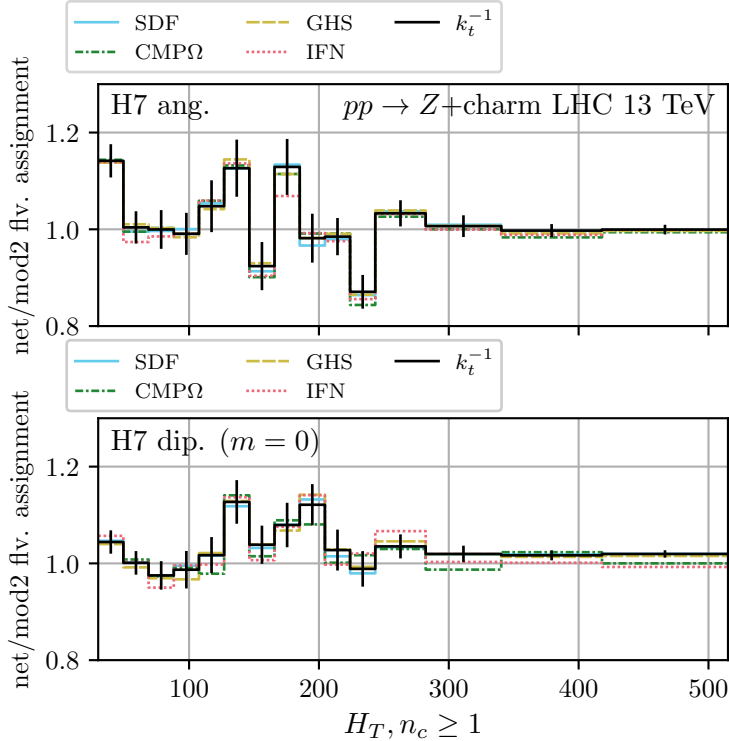

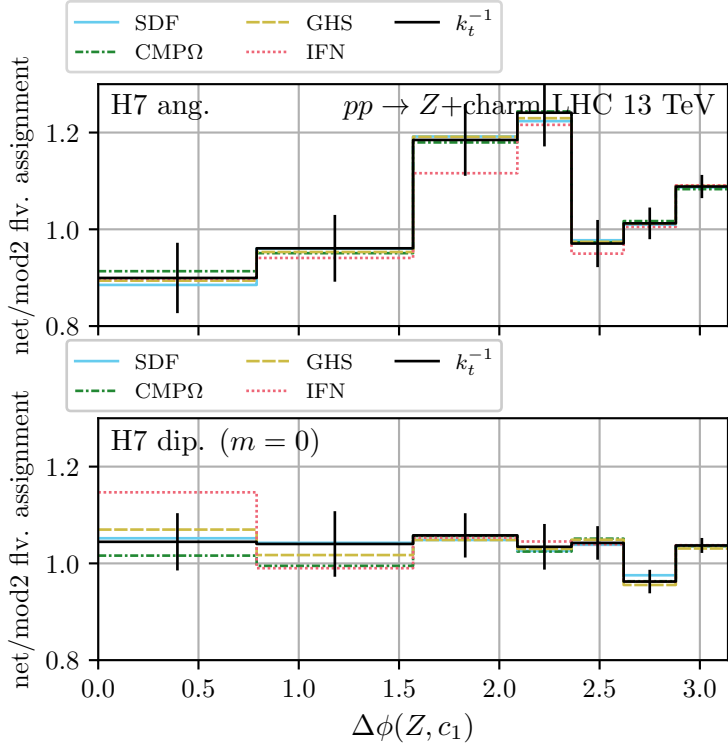

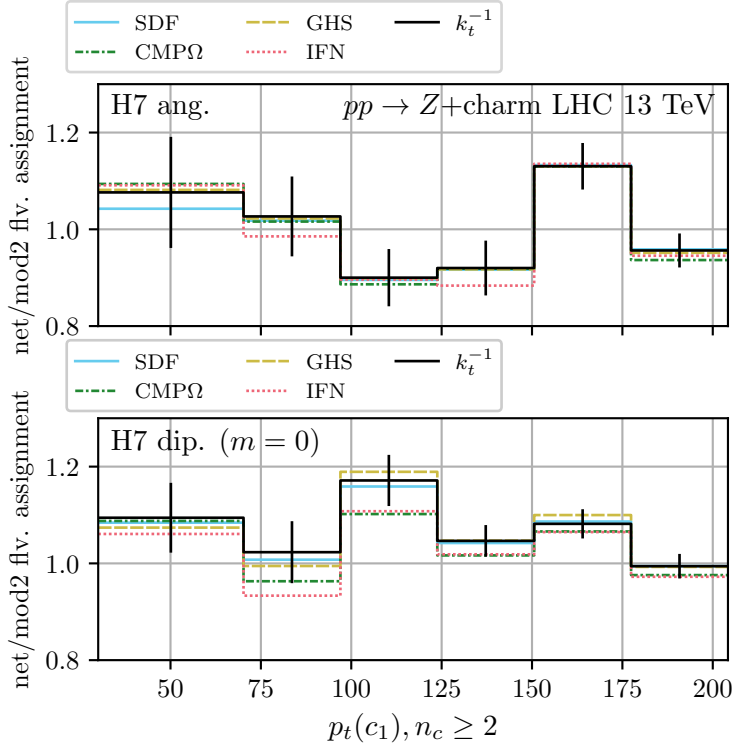



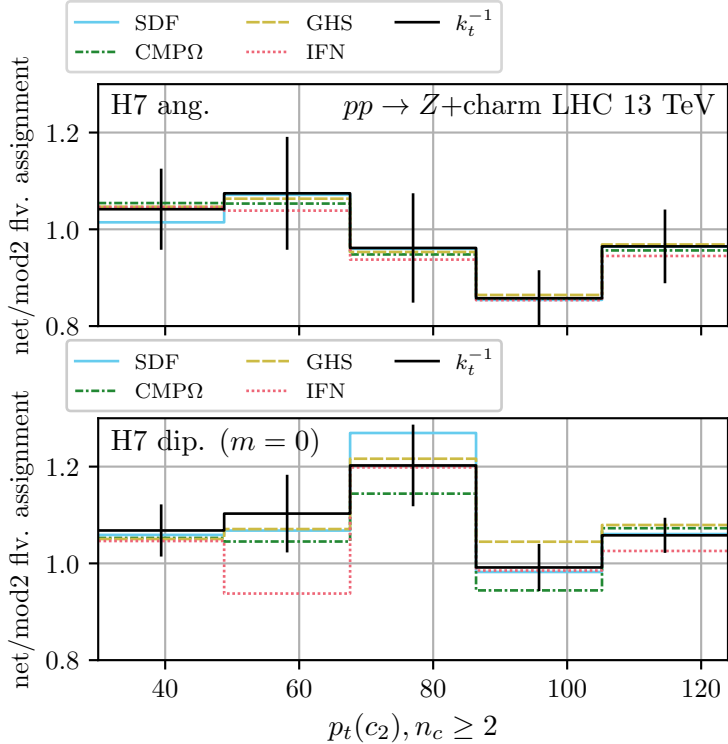

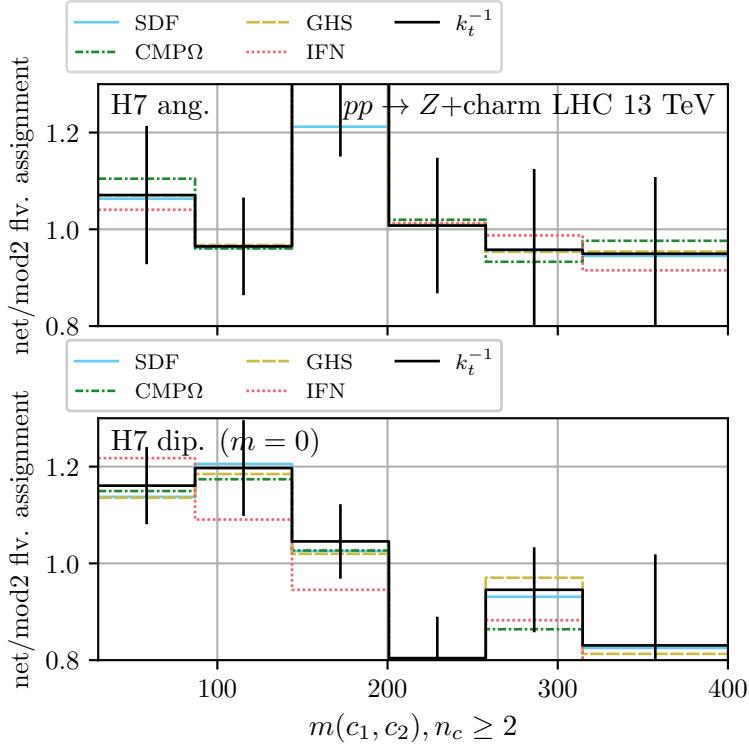

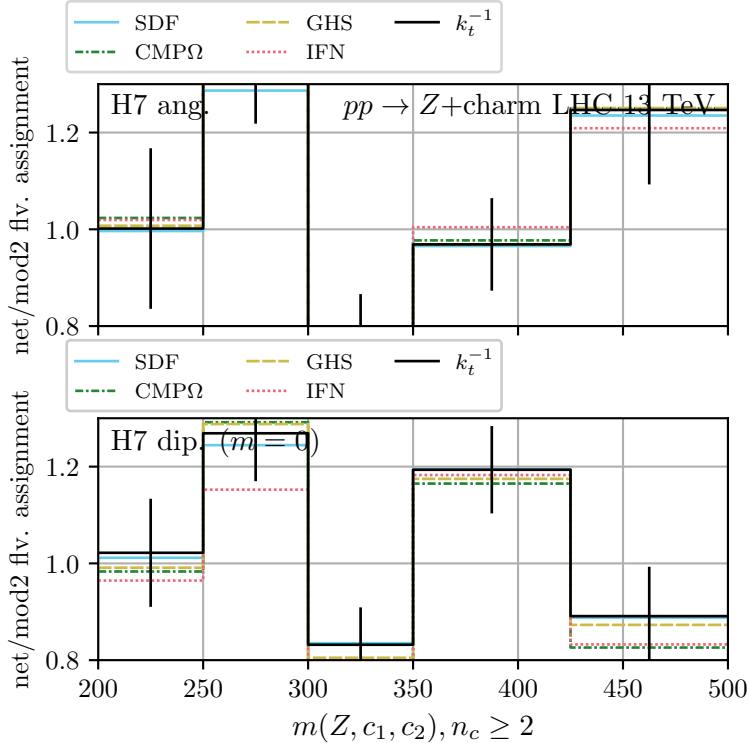

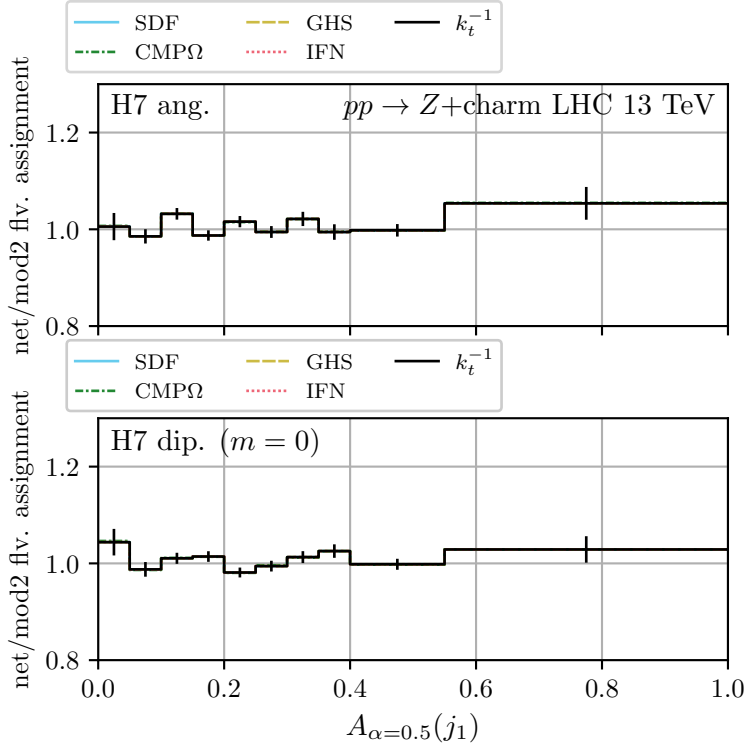

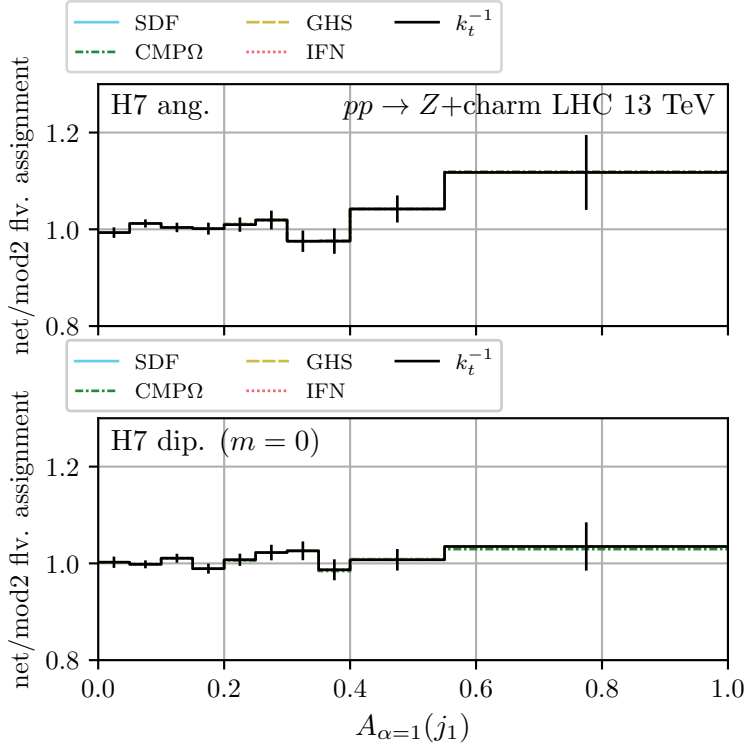

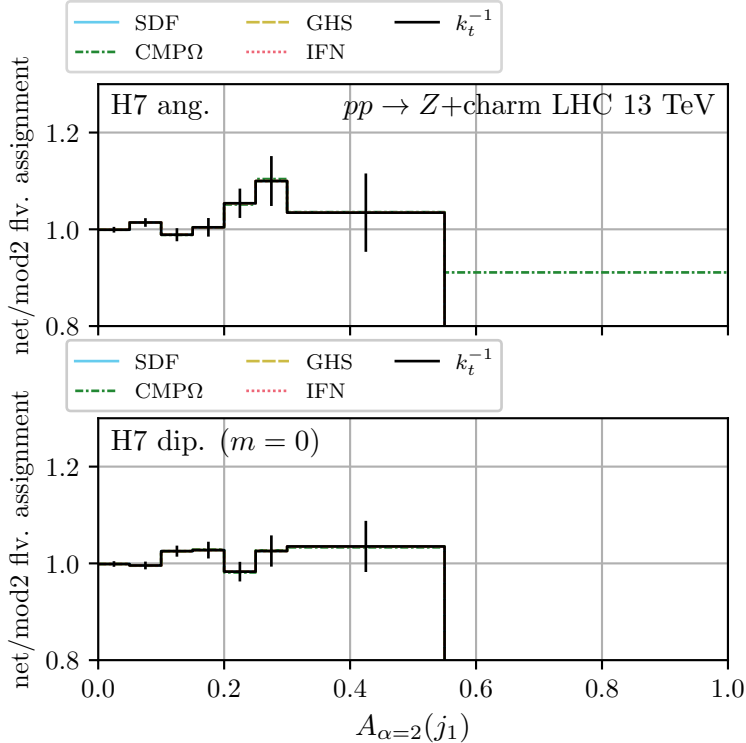

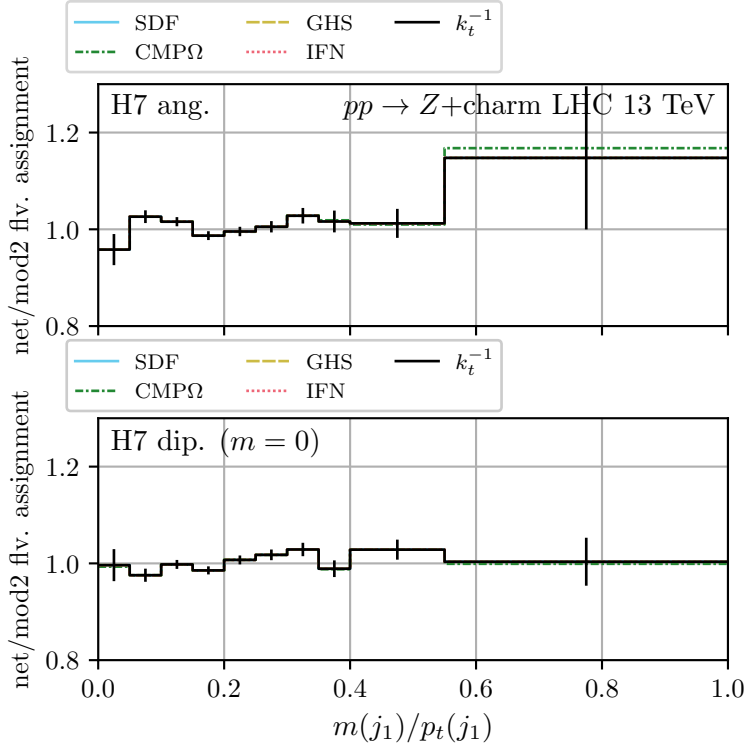

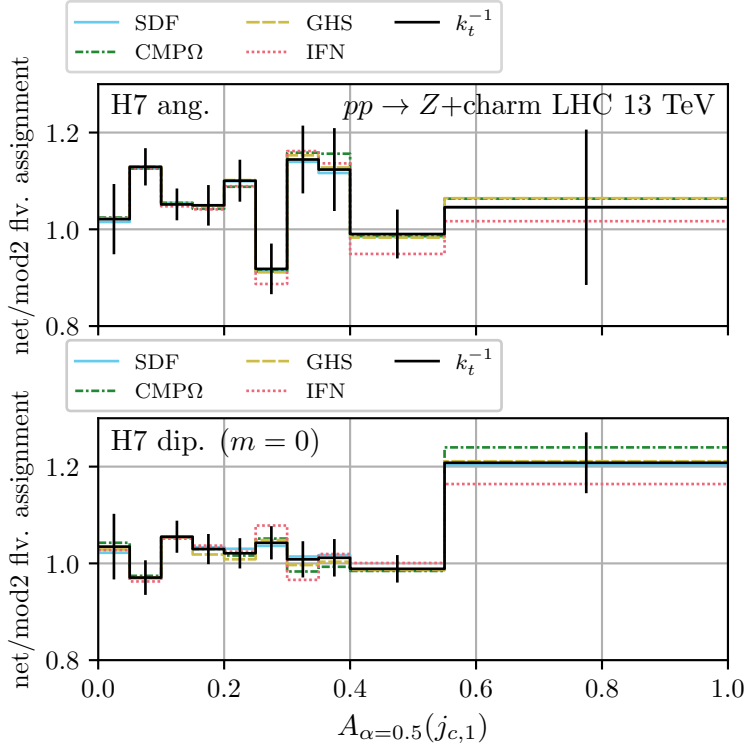



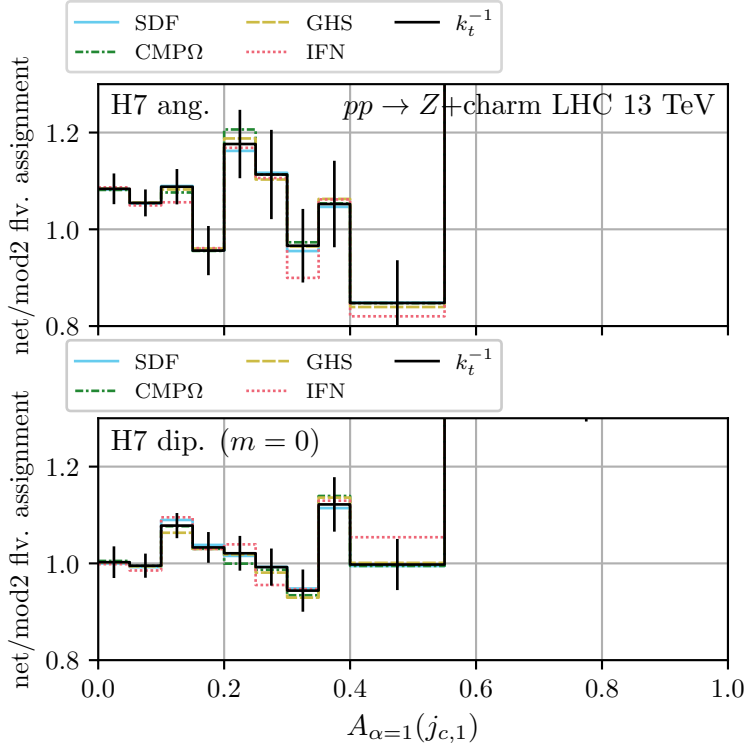

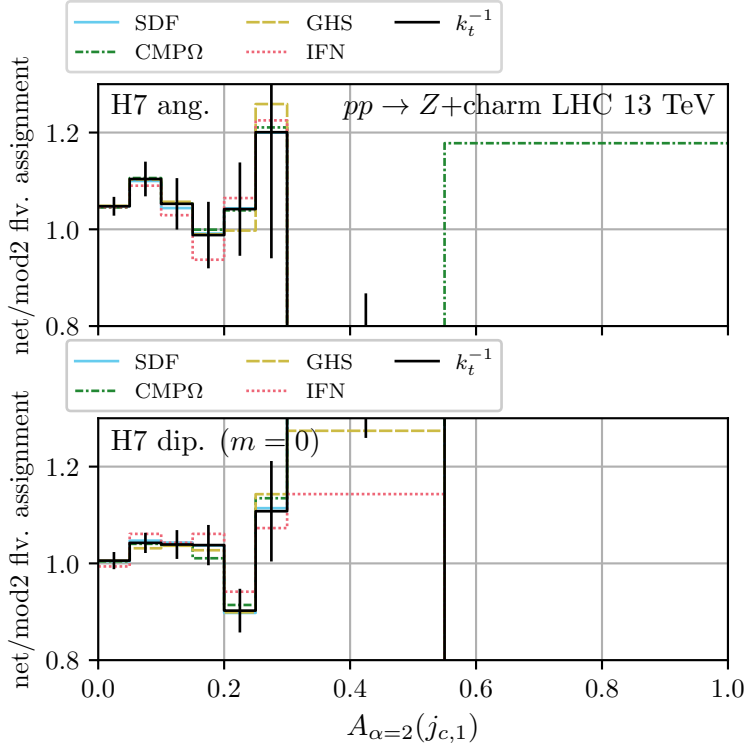

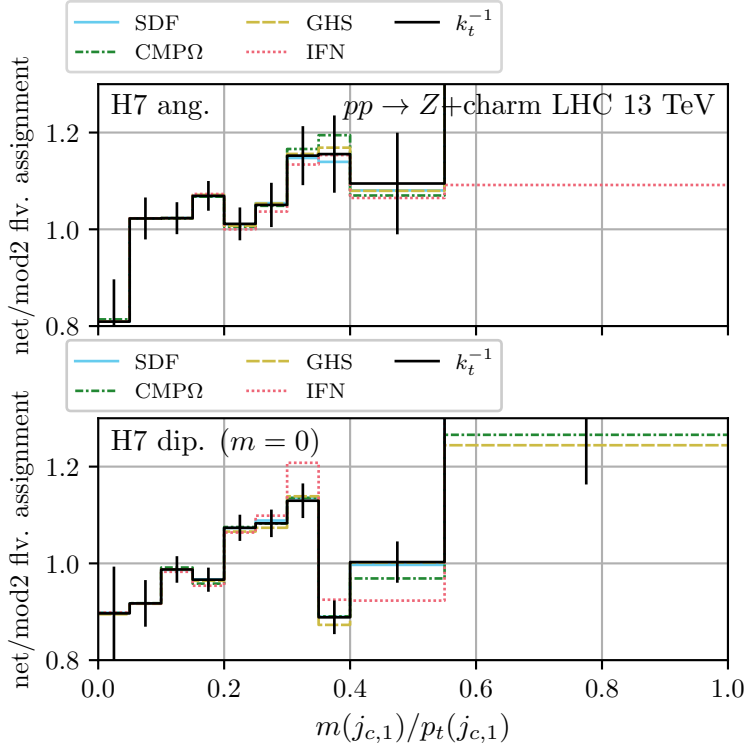

Supplement: Supplementary file 4 [file ppzj_charm_nlops_comparisons_appendix_netflv.pdf]
